# Supplementary material for: Semi-Automated Modular Formal Verification of Critical Software: Liveness and Completeness Thresholds
Source: arXiv:2403.00934 source file (2024-03-14)
Supplement: Supplementary file 6 [file ctms--stable_memory.tex]

\documentclass[../ct4ms-TR-CAV.tex.tex]{subfiles}

\begin{document}

%\NewDocumentCommand{\keyword}{m}{\texttt{#1}}

% TODO: move to package and include package in main file

\end{document}
