# Supplementary material for: Semi-Automated Modular Formal Verification of Critical Software: Liveness and Completeness Thresholds
Source: arXiv:2403.00934 source file (2024-03-14)
Supplement: Supplementary file 8 [file sec-MS-CT-combinators.tex]

\documentclass[../ct4ms-TR-CAV.tex]{subfiles}

\begin{document}

\begin{lemma}[Sequence Combinator]
		Let $\cstSetVar_1, \cstSetVar$ be constraint sets describing the completeness thresholds for \varVar in  
		\msHoareTriple{A}{\cmdVar_1}[\resVar]{B} 
		and
		\msHoareTriple{B}{\cmdVar_2}[\resVar']{C},
		respectively.
		Then $\cstSetVar_1 \cup \cstSetVar_2$ is a completeness threshold for \varVar in
		\msHoareTriple{A}{\cmdVar_1; \cmdVar_2}{C}.
\end{lemma}
\begin{proof}
	content
	
	\revProblem{I think this is false}
\end{proof}

Goal: We want to find a way to compute a CT for
\msHoareTriple{\preVar}{\cmdVar_1; \cmdVar_2}{\preVar}
from CTs for $\cmdVar_i$.

\TodoTextNote{
	\begin{itemize}
		\item Extend syntax by assert commands.
		\item Extend dynamic semantics by assert commands.
		\item Add assertion errors. Should we introduce a new kind of error to differentiate between memory and assertion errors?
		\item Extend Hoare triple definition and memory safety definition to include assertion errors.
		\item Define substitution for Hoare triples.
	\end{itemize}
}

\revRemark{
	For now, we imagine that \cmdAssert{...} throws an error and that "memsafe(..., c)" means no ERROR gets thrown.
}

\TodoTextNote{Should we call it rule of consequence?}
\begin{lemma}[Hoare Triple Sequence]\label{genCTsTR:appendix:lem:HoareTripleSequence}
$$
	\begin{array}{l}
		\mshtValid{A}{\cmdVar_1}{B}
		\ \ \wedge\
		\mshtValid{C}{\cmdVar_2}{D}
		\ \ \wedge\
		\assValid{B \rightarrow C}
		\\
		\Longrightarrow\quad
		\msHoareTriple
			{A}
			{\cmdVar_1; \cmdAssert{B}; \cmdVar_2}
			{D}
	\end{array}
$$
\end{lemma}
\begin{proof}
	\TodoTextNote{Prove}
\end{proof}

\begin{lemma}[Invariant Assertion Sequence]\label{genCTsTR:appendix:lem:invariantAssertionSequence}
$$
	\mshtValid
		{\preVar}
		{\cmdVar_1; \cmdAssert{\preVar}; \cmdVar_2}
		{\preVar}
	\quad\Longleftrightarrow\quad
	\bigwedge_{i=1,2}
		\mshtValid
			{\preVar}
			{\cmdVar_i}
			{\preVar}	
$$
\end{lemma}
\begin{proof}
	\TodoTextNote{Prove}
\end{proof}

\begin{lemma}[Stable Sequence Combinator]
	For $i=1, 2$, let $\ctVar_i$ be completeness thresholds for \varVar in
	\msHoareTriple{\preVar}{\cmdVar_i}{\preVar},
	respectively.
	Then $\ctVar_1 \cup \ctVar_2$ is a completeness threshold for \varVar in
	\msHoareTriple
		{\preVar}
		{\cmdVar_1; \cmdAssert{\preVar}; \cmdVar_2}
		{\preVar}.
\end{lemma}
\begin{proof}
	Suppose
	$\forall \varVar \in \ctVar_1 \cup \ctVar_2.\
		\mshtValid
			{\preVar}
			{\cmdVar_1; \cmdAssert{\preVar}; \cmdVar_2}
			{\preVar}
	$
	holds.
	By Lem.\ref{genCTsTR:appendix:lem:invariantAssertionSequence} we get
	$\forall \varVar \in \ctVar_1 \cup \ctVar_2.\
		\mshtValid
			{\preVar}
			{\cmdVar_i}
			{\preVar}
	$.
	Since $\ctVar_i$ are completeness thresholds for \varVar,
	this implies
	\mshtValid
		{\preVar}
		{\cmdVar_i}
		{\preVar}.
	By Lem.~\ref{genCTsTR:appendix:lem:HoareTripleSequence}
	we get
	\mshtValid
		{\preVar}
		{\cmdVar_1; \cmdAssert{\preVar}; \cmdVar_2}
		{\preVar}
	and hence $\ctVar_1 \cup \ctVar_2$ is a completeness threshold for \varVar in 
	\msHoareTriple
		{\preVar}
		{\cmdVar_1; \cmdAssert{\preVar}; \cmdVar_2}
		{\preVar}.
\end{proof}

\end{document}
