# Supplementary material for: Semi-Automated Modular Formal Verification of Critical Software: Liveness and Completeness Thresholds
Source: arXiv:2403.00934 source file (2024-03-14)
Supplement: Supplementary file 10 [file sec-constraints.tex]

\documentclass[../ct4ms-TR-CAV.tex]{subfiles}

\begin{document}

\TodoTextNote{
	\begin{itemize}
		\item Formulate the idea behind constraints (connection to equivalence covers and Equivalence Cover Lem.~\ref{genCTsTR:appendix:theo:eqCoverCT}, CT Extraction Cor~\ref{genCTsTR:appendix:corollary:CTextraction} )
	\end{itemize}
}

We use a propositional logic enriched with program expressions to express constraints.

\begin{definition}[Constraint Syntax]
	We define the set of constraints $\cstVar \in \ConstraintSet$ syntactically by the grammar presented in Fig.~\ref{genCTsTR:appendix:fig:def:Constraints}.
\end{definition}

\begin{figure}
	\begin{subfigure}{\textwidth}
		$$
		\begin{array}{l l l}
			\expVar \in \ExpSet
			\\
			\cstVar \in \ConstraintSet
				&:=
				& \slTrue \alt \slFalse \alt
					\expVar \alt
					\neg \cstVar \alt
					\cstVar \wedge \cstVar
		\end{array}
		$$
		\caption{Constraint syntax.}
	\end{subfigure}
	
	\begin{subfigure}{\textwidth}
		$$
		\begin{array}{l l l}
			\cstVar_1 \vee \cstVar_2
				&:=
				&\neg( \neg\cstVar_1 \wedge \neg\cstVar_2)
			\\
			\cstVar_1 \rightarrow \cstVar_2
				&:=
				&\neg \cstVar_1 \vee \cstVar_2
			\\
			\cstVar_1 \leftrightarrow \cstVar_2
				&:=
				&(\cstVar_1 \rightarrow \cstVar_2)
					\wedge
					(\cstVar_2 \rightarrow \cstVar_1)
		\end{array}
		$$
		\caption{Syntactic sugar.}
	\end{subfigure}
	
	\caption{Constraints.}
	\label{genCTsTR:appendix:fig:def:Constraints}
\end{figure}

\begin{definition}[Constraint Model Relation]
	We define a model relation for constraints
	$\cstModelsSymb\ 
		\subseteq 
		(\VarSet \rightarrow \ValueSet)
		\times
		\ConstraintSet
	$
	by recursion over the structure of constraints according to the rules presented in Fig.~\ref{genCTsTR:appendix:fig:def:ConstraintModelRelation}.
	We denote interpretations mapping variable symbols to values by \interpretationVar.
\end{definition}

We extend interpretations of variables to interpretations of expressions in the canonical way.

\begin{definition}[Extending Interpretations to Expressions]
	For  any interpretation
	$\interpretationVar: \VarSet \rightarrow \ValueSet$
	of variables,
	the canonical extension to expressions is
	$\interpretationVar: \ExpSet \rightarrow \ValueSet$
	with
	$$
		\interpretationVar(\expVar)
		=
		\evalExp
		{
			\subst
			{
				\subst
				{\expVar}
				{\varVar_1}
				{\interpretationVar(\varVar_1)}
				\dots
			}
			{\varVar_n}
			{\interpretationVar(\varVar_n)}
		}
	$$
	where
	$\freeVars[\expVar] = \setOf{\varVar_1, \dots, \varVar_n}$.
\end{definition}

\begin{figure}
	$$
	\begin{array}{l l l}
		\cstModels{\interpretationVar}{\slTrue}
		\\
		\cstNotModels{\interpretationVar}{\slFalse}
		\\
		\cstModels{\interpretationVar}{\expVar}
			&\text{iff}
			&\cstModels
				{\emptyset}
				{\interpretationVar(\expVar)}
		\\
		\cstModels{\interpretationVar}{\neg\cstVar}
			&\text{iff}
			&\cstNotModels{\interpretationVar}{\cstVar}
		\\
		\cstModels
			{\interpretationVar}
			{\cstVar_1 \wedge \cstVar_2}
			&\text{iff}
			&\cstModels{\interpretationVar}{\cstVar_1}
				\ \text{and}\
				\cstModels{\interpretationVar}{\cstVar_2}
	\end{array}
	$$
	\TodoTextNote{Define constraint model relation}
	\caption{Constraint model relation. We write \cstNotModels{\interpretationVar}{\cstVar} if \cstModels{\interpretationVar}{\cstVar} does not hold.}
	\label{genCTsTR:appendix:fig:def:ConstraintModelRelation}
\end{figure}

\revQuestion{Do we need to support constraints with multiple free vars?}

\begin{definition}[Existential Constraint Model Relation]
	We define the model relation 
	$\exCstModelsSymb\
		\subseteq 
		\powerSetOf{\ValueSet} 
		\times
		\ConstraintSet
	$
	as follows
	$$
		\exCstModels{\domVar}{\cstVar}
		\quad\Leftrightarrow\quad
		\exists \varVar.\ 
		\exists \valVar \in \domVar.\
			\freeVars[\cstVar] = \setOf{\varVar}
		\wedge
			\cstModels
				{\setOf{\varVar \mapsto \valVar}}
				{\cstVar}
	$$.
	We write \exCstNotModels{\domVar}{\cstVar} if \exCstModels{\domVar}{\cstVar} does not hold.
	We say that \domVar complies with the constraint \cstVar or that \cstVar describes \domVar if \exCstModels{\domVar}{\cstVar} holds.
\end{definition}

\begin{definition}[Existential Constraint Set Model Relation]
	We extend the existential constraint model relation 
	$\exCstModelsSymb\
		\subseteq 
		\powerSetOf{\ValueSet} 
		\times
		\ConstraintSet
	$
	to one over constraint sets 
	$\exCstModelsSymb\
		\subseteq 
		\powerSetOf{\ValueSet} 
		\times
		\powerSetOf{\ConstraintSet}
	$
	as follows:
	$$
		\exCstModels{\domVar}{\cstSetVar}
		\quad\Leftrightarrow\quad
		\bigwedge_{\cstVar \in \cstSetVar}
			\exCstModels{\domVar}{\cstVar}.
	$$
	We denote constraint sets by $\cstSetVar \subseteq \ConstraintSet$.
\end{definition}

\end{document}
