# Supplementary material for: Semi-Automated Modular Formal Verification of Critical Software: Liveness and Completeness Thresholds
Source: arXiv:2403.00934 source file (2024-03-14)
Supplement: Supplementary file 14 [file sec-memory_safety.tex]

\documentclass[../ct4ms-TR-CAV.tex]{subfiles}

\begin{document}

We consider a command memory safe under a heap if its execution does not lead to a memory error.

\begin{definition}[Memory Safety of Commands and Heaps]
	We define the memory safety relation for commands 
	$\memSafeCmdHeapName \subseteq \PhysHeapSet \times \CmdSet$ 
	as follows:
	
	Let 
	$\overline{\varVar} = (\varVar_i)_i 
	\congruent
	\freeVars[\cmdVar]
	$
	be the variables occurring freely in \cmdVar.
	For each~$i$, let $\typeVar_i$ be the type of variable $\varVar_i$ and let $\overline{\typeVar} = (\typeVar_i)_i$.
	Then,
	$$
	\memSafeCmdHeap{\pheapVar}{\cmdVar}
	\ \Leftrightarrow \
	\forall \overline{\valVar} \in \overline{\typeVar}.\
	\neg\exists \nextPheapVar.\
	\cmdRedStepStar
	[\pheapVar]
	{\subst
		{\cmdVar}
		{\overline{\varVar}}
		{\overline{\valVar}}
	}
	[\nextPheapVar]
	{\memoryError}
	$$
	We say that a command \cmdVar is \emph{memory safe} under a physical heap \pheapVar if \memSafeCmdHeap{\pheapVar}{\cmdVar} holds.
\end{definition}

Note that this definition allows a command's execution to get stuck as long as no memory error occurs.
Such cases arise for not-well-typed commands such as \cmdIfNoElse{13}{\dots}.
For this work, we only consider well-typed programs.
Hence, we do not care about cases in which a program gets stuck as long as no memory error occurs. Moreover, we consider a command to be memory safe under a precondition \preVar if it is memory safe under any heap \pheapVar that complies with the precondition, i.e.
$\assModels{\pheapVar}{\preVar}$.

\begin{definition}[Memory Safety of Commands and Assertions]
	\label{genCTsTR:appendix:def:memorySafetyAss}
	We define the memory safety relation for commands 
	$\memSafeCmdAssName \subseteq \AssertionSet \times \CmdSet$ 
	as follows:
	
	Let 
	$\overline{\varVar} = (\varVar_i)_i 
	\congruent
	\freeVars[\assVar, \cmdVar]
	$
	be the variables occurring freely in \assVar and \cmdVar.
	For each~$i$, let $\typeVar_i$ be the type of variable $\varVar_i$ and let $\overline{\typeVar} = (\typeVar_i)_i$.
	Then,
	$$
	\memSafeCmdAss{\assVar}{\cmdVar}
	\quad \Longleftrightarrow \quad
	\forall \overline{\valVar} \in \overline{\typeVar}.\
	\forall \pheapVar.\
	\big(
	\assModels
	{\pheapVar}
	{\subst
		{\assVar}
		{\overline{\varVar}}
		{\overline{\valVar}}
	}
	\ \Rightarrow\
	\memSafeCmdHeap
	{\pheapVar}
	{\subst
		{\cmdVar}
		{\overline{\varVar}}
		{\overline{\valVar}}
	}
	\big)
	$$
	We say that a command \cmdVar is \emph{memory safe} under an assertion \assVar if \memSafeCmdAss{\assVar}{\cmdVar} holds.
\end{definition}

\begin{observation}
	For any fixed assertion \assVar, 
	the relation 
	$\memSafeCmdAss{\assVar}{\cmdVar} \subseteq \CmdSet$
	is a correctness property.
\end{observation}

We use Hoare triples to express program specifications.
Following the intuition formalized in Def.~\ref{genCTsTR:appendix:def:memorySafetyAss}, we only consider program runs erroneous if they lead to a memory error.
In the language we consider, the only other reason for a run being stuck is that the program is not well-typed.
To highlight that our definition of Hoare triples differs in this respect from the common definitions, we write
\msHoareTriple{\preVar}{\cmdVar}[\resVar]{\postVar}
instead of 
\hoareTriple{\preVar}{\cmdVar}[\resVar]{\postVar}.

For us, a memory safety Hoare triple
\msHoareTriple{\preVar}{\cmdVar}[\resVar]{\postVar}
expresses two points:
\begin{itemize}
	\item The command \cmdVar is memory safe under the precondition \preVar.
	That is, when \cmdVar is executed under any heap that models the precondition, the execution does not lead to a memory error.
	\item If the execution of \cmdVar under precondition \preVar terminates successfully, i.e., if \cmdVar reduces to a value \valVar, then postcondition \subst{\postVar}{\resVar}{\valVar} holds in the final state.
\end{itemize}

\begin{definition}[Model Relation for Memory Safety Hoare Triples]
	Let $\preVar, \postVar$ be assertions and \cmdVar a command.
	Let 
	$\overline{\varVar} = (\varVar_i)_i 
		\congruent
		\freeVars[\preVar, \cmdVar, \postVar]
	$
	be the variables occurring freely in \preVar, \cmdVar, \postVar.
	For each~$i$, let $\typeVar_i$ be the type of variable $\varVar_i$ and let $\overline{\typeVar} = (\typeVar_i)_i$.
	We define the model relation for memory safety Hoare triples
	$\htModelsSymb
		\ \subseteq\
		\AssertionSet \times \CmdSet \times 
			(\ValueSet \rightarrow \AssertionSet)
	$
	as follows:
	$$
	\begin{array}{c}
		\mshtValid{\preVar}{\cmdVar}[\resVar]{\postVar}
		\\
		\Longleftrightarrow
		\\
		\begin{array}{ll}
		(
			\memSafeCmdAss{\preVar}{\cmdVar}
			\ \wedge\!\!
			&(
				\forall \overline{\valVar} \in \overline{\typeVar}.\
				\forall \pheapVar_\preVar.\
					\assModels
						{\pheapVar_\preVar}
						{\subst{\preVar}
							{\overline{\varVar}}
							{\overline{\valVar}}
						}
					\ \rightarrow
		\\
		&\phantom{
			\forall \overline{\valVar} \in \overline{\typeVar}.\
			\forall \pheapVar_\preVar.\
		}\
				(
					\exists \pheapVar_\postVar.\
					\exists \valVar'.\
						\cmdRedStepStar
							[\pheapVar_\preVar]
							{\subst
									{\cmdVar}
									{\overline{\varVar}}
									{\overline{\valVar}}
							}
							[\pheapVar_\postVar]
							{\valVar'}
							\ \rightarrow
		\\
		&\phantom{
			\forall \overline{\valVar} \in \overline{\typeVar}.\
			\forall \pheapVar_\preVar.\
			\exists \pheapVar_\postVar.\
			\exists \valVar'.\
		}\ \
						\assModels
							{\pheapVar_\postVar}
							{\subst
								{\postVar}
								{\overline{\varVar}, \resVar}
								{\overline{\valVar}, \valVar'}
							}
				)
			)
		)
		\end{array}
	\end{array}
	$$
	For convenience of notation we define
	$$
		\mshtValid{\preVar}{\cmdVar}{\postVar}
		\ \Longleftrightarrow\ \
		\mshtValid{\preVar}{\cmdVar}[y]{\postVar}
	$$
	for any $y \not\in \freeVars({\postVar})$.
\end{definition}

\begin{observation}
	For any fixed pre and postcondition \preVar and \postVar, 
	the relation 
	$\msHoareTriple{\preVar}{\cmdVar}[\resVar]{\postVar} \subseteq \CmdSet$
	is a correctness property.
\end{observation}

\begin{remark}
	Note that for any canonical type system and for any well typed command \cmdVar, 
	the canonical Hoare triple
	\hoareTriple{\preVar}{\cmdVar}[\resVar]{\postVar}
	would be equivalent to our 
	memory safety Hoare triple
	\msHoareTriple{\preVar}{\cmdVar}[\resVar]{\postVar}.
\end{remark}

\begin{corollary}
	Let \assVar be an assertion and \cmdVar a command.
	Then
	$$
	\mshtValid{\assVar}{\cmdVar}{\slTrue}
		\ \Leftrightarrow\
		\memSafeCmdAss{\assVar}{\cmdVar}
		.
	$$
\end{corollary}
\begin{proof}
	$$
	\begin{array}{l}
		\mshtValid{\assVar}{\cmdVar}{\slTrue}
		\\
		\Longleftrightarrow
		% ---------------------------------
		% Instantiate B with true
		\begin{array}[t]{ll}
			\memSafeCmdAss{\preVar}{\cmdVar}
			\ \wedge\!\!
			&(\forall \overline{\valVar} \in \overline{\typeVar}.\
			\forall \pheapVar_\preVar.\
			\assModels
				{\pheapVar_\preVar}
				{\subst{\preVar}
					{\overline{\varVar}}
					{\overline{\valVar}}
				}
			\ \rightarrow
		\\
		&\phantom{
			\forall \overline{\valVar} \in \overline{\typeVar}.\
			\forall \pheapVar_\preVar.\
		}\
			(
				\exists \pheapVar_\postVar.\
				\exists \valVar'.\
				\cmdRedStepStar
					[\pheapVar_\preVar]
					{\subst
						{\cmdVar}
						{\overline{\varVar}}
						{\overline{\valVar}}
					}
					[\pheapVar_\postVar]
					{\valVar'}
		\\
		&\phantom{
			\forall \overline{\valVar} \in \overline{\typeVar}.\
			\forall \pheapVar_\preVar.\
			\exists \pheapVar_\postVar.\
			\exists \valVar'.\
		}\ \
				\rightarrow\
				\assModels
					{\pheapVar_\postVar}
					{\slTrue}
			)
			)
		\end{array}
		\\
		\Longleftrightarrow
		% ---------------------------------
		% Simplify inner implication
		\begin{array}[t]{ll}
			\memSafeCmdAss{\preVar}{\cmdVar}
			\ \wedge\!\!
			&(\forall \overline{\valVar} \in \overline{\typeVar}.\
			\forall \pheapVar_\preVar.\
			\assModels
				{\pheapVar_\preVar}
				{\subst{\preVar}
					{\overline{\varVar}}
					{\overline{\valVar}}
				}
			\ \rightarrow\
			\slTrue
			)
		\end{array}		
		\\
		\Longleftrightarrow
		% ---------------------------------
		% Simplify outer implication
		% Note: We keep the array to ensure that the 
		%       spacing remains consistent
		\begin{array}{l}
			\memSafeCmdAss{\preVar}{\cmdVar}
			\ \wedge\
			\slTrue
		\end{array}
	\end{array}
	$$
\end{proof}

We use weakest liberal preconditions~\cite{Flanagan2001AvoidingExpExplosionVC, Dijsktra1976DisciplineOfProgramming} as verification conditions.
In order to compute them, we first have to annotate loop commands with loop invariants.

\begin{definition}[Annotated Commands]
	We define the set of annotated commands \AnnotCmdSet syntactically by the grammar presented in Fig.~\ref{genCTsTR:appendix:fig:def:AnnotatedCommandSyntax}.
	The omitted rules are analogous to the standard syntax grammar rules presented in Fig.~\ref{genCTsTR:appendix:fig:def:ProgSyntax}.
\end{definition}

\begin{figure}
	$$
	\begin{array}{lcl p{0.0cm}l}
	\\
	\varVar  \in  \VarSet
		&&&&\text{Variables}
	\\
	\expVar \in \ExpSet
		&&&&\text{Expressions}
	\\
	\assVar \in \AssertionSet
		&&&&\text{Assertions}
	\\
	\annotCmdVar \in \AnnotCmdSet &::= 
	&\dots \alt
	\\
	&&\cmdWhileInv{\cmdReadHloc{\expVar}}{\assVar}{\annotCmdVar}
		\alt
		&&\text{Loops annotated}
	\\
	&&\cmdForInv{\varVar}{\rangeFromTo{\expVar}{\expVar}}{\assVar}{\annotCmdVar}
		\alt
		&&\text{with invariants}
	\\
	&&\dots
	\end{array}
	$$

	\caption{Syntax of annotated commands.}
	\label{genCTsTR:appendix:fig:def:AnnotatedCommandSyntax}
\end{figure}

\TodoTextNote{Define annotation relation}

\begin{definition}[Assertion Lambdas]
	We define the set of assertion lambda terms as
	$\AssertionLambdaSet :=
	\setOf
	[\lambda \varVar.\ \assVar]
	{\varVar \in \VarSet, \assVar \in \AssertionSet}
	$.
	For convenience we define the notation
	$\lambdaIgnore{\assVar} := \lambda \varVar_{fresh}.\ \assVar$
	for $\varVar_{fresh} \not\in \freeVars[\assVar]$.
\end{definition}

We use assertion lambda terms $\lambda \resVar. \postVar$ to denote postconditions referring to a result value \resVar.

\begin{definition}[Weakest Liberal Precondition]
	We define the weakest liberal precondition function 
	$wlp : \AnnotCmdSet \times \AssertionLambdaSet \rightarrow \AssertionSet$
	by recursion over the structure of commands as follows:
	$$
	\begin{array}{l c l}
	wlp(\expVar,\ \lambda\resVar.\ \postVar)
	&:=
	&\subst{\postVar}{\resVar}{\expVar},
	\\
	wlp(
	\cmdLet{\varVar}{\cmdVar_1}{\cmdVar_2},\
	\lambda \resVar.\ \postVar
	)
	&:=
	&wlp(
	\cmdVar_1,\ 
	\lambda \varVar.\ 
	wlp(\cmdVar_2,\ \lambda \resVar.\ \postVar)
	),
	\\
	wlp(
	\cmdIf{\expVar}{\cmdVar_t}{\cmdVar_f},\
	\lambda \resVar.\ \postVar
	)
	&:=
	&(\expVar 
	\rightarrow 
	wlp(\cmdVar_t,\ \lambda \resVar.\ \postVar)
	)
	\\
	&&
	\wedge\
	(\neg\expVar 
	\rightarrow 
	wlp(\cmdVar_f,\ \lambda \resVar.\ \postVar)
	),
	\\
	wlp(\cmdWhileInv{\cmdReadHloc{\expVar}}{\invVar}{\cmdVar}, 
	\lambda \resVar.\ \postVar
	)
	&:=
	&\invVar
	\\
	&&\slStar\
	\slPersistent(
	\invVar \ \slWand\ \slPointsTo{\expVar}{\slWildcard}
	)
	\\
	&&\slStar\ 
	\slPersistent (
	\invVar \wedge \slPointsTo{\expVar}{\slTrue} 
	\ \slWand\
	wlp(\cmdVar, \lambdaIgnore{\invVar})
	)
	\\
	&&\slStar\ 
	(
	\invVar \wedge \slPointsTo{\expVar}{\slFalse} 
	\ \slWand\
	\postVar
	),
	\\
	wlp(\cmdForInv
	{\varVar}
	{\rangeFromTo{\expVar_1}{\expVar_2}}
	{\invVar}
	{\cmdVar},
	&:=
	&\invVar
	\\
	\phantom{wlp(}
	\lambda \resVar.\ \postVar)
	&&\slStar\
	\slPersistent(
	\forall \varVar.\ 
	\expVar_1 \leq \varVar < \expVar_2
	\wedge
	\invVar
	\ \slWand\
	wlp(\cmdVar, \lambdaIgnore{\invVar})
	)
	\\
	&&\slStar\
	(\invVar \ \slWand\ \postVar),
	\\
	wlp(\cmdReadHloc{\expVar}, \lambda \resVar.\ \postVar)
	&:=
	&\exists y.\ 
	\slPointsTo{\expVar}{y}
	\wedge
	\subst{\postVar}{\resVar}{y}
	\\
	&&\text{where}\quad
	y \not\in \freeVars[\expVar, \postVar],
	%		\\
	%		&&
	\revRemark[Alternative wlp]
	{$
		\exists y.\
		\slPointsTo{\expVar}{y}
		\slStar
		(
		\slPointsTo{\expVar}{y}
		\slWand
		\subst{\postVar}{\resVar}{y}
		)
		$}
	\\
	wlp(\cmdAssignHloc{\expVar_1}{\expVar_2}, \lambda\resVar.\ \postVar)
	&:=
	&\slPointsTo{\expVar_1}{\slWildcard}
	\ \slStar\
	(
	\slPointsTo{\expVar_1}{\expVar_2}
	\slWand
	\postVar
	),
	\\
	wlp(\hCmdVar(\overline{\expVar}), \lambda\resVar.\ \postVar)
	&:=
	&wlp(
	\subst
	{\bCmdVar}
	{\overline{\varVar}}
	{\overline{\expVar}},
	\lambda \resVar.\ \postVar)
	\\
	&&\text{where}\quad
	\hcmdInterpret[\hCmdVar] = (\bCmdVar, \overline{\varVar})
	\end{array}
	$$
\end{definition}

Note that our weakest precondition for \keyword{for} loops does not allow the postcondition to depend on the knowledge that any work was done.
This simplified precondition is sufficient to reason about the memory safety of array-traversing programs that do not allocate nor free memory.

\begin{lemma}[WLP for Syntactic Sugar]
	$$
	\begin{array}{l c l}
		wlp(\cmdVar; \nextCmdVar,\ \lambda\resVar.\ \postVar)
			&\equiv
			&wlp(\cmdVar,\ \lambda\slWildcard.\ 
					wlp(\nextCmdVar,\ \lambda\resVar.\ \postVar)
			)
		\\
		wlp(\cmdAssignHloc
					{\expVar}
					{\cmdReadHloc{\nextExpVar}},\
				\lambda\resVar.\ \postVar
		)
		&\equiv
		&\exists y.\
				\slPointsTo{\nextExpVar}{y}
				\ \wedge\ 
				(
					\slPointsToAny{\expVar} 
					\ \slStar\
					(\slPointsTo{\expVar}{y} \slWand \postVar)
				)
		\\
		&&\text{where $y$ is not free in \varVar, \expVar, \nextExpVar, \postVar}
		\\
		wlp(\cmdAssignHloc
					{\expVar}
					{\cmdReadHloc{\expVar}},\
				\lambda\resVar.\ \postVar
			)
		&\equiv
		&\exists y.\
			\slPointsTo{\expVar}{y}\ \wedge\ \postVar
	\end{array}
	$$
\end{lemma}
\begin{proof}
	$$
	\begin{array}{l l l}
		&wlp(\cmdVar; \nextCmdVar,\ \lambda\resVar.\ \postVar)
		&\text{\varVar not fresh in \nextCmdVar}
		\\
		=
		&wlp(\cmdLet{\varVar}{\cmdVar}{\nextCmdVar},\ 
					\lambda\resVar.\ \postVar
			)
		\\
		=
		&wlp(\cmdVar, 
					\lambda\varVar.\ 
						wlp(\nextCmdVar,\ \lambda\resVar.\ \postVar)
			)
		\\
		\equiv
		&wlp(\cmdVar, 
			\lambda\slWildcard.\ 
			wlp(\nextCmdVar,\ \lambda\resVar.\ \postVar)
		)
	\end{array}
	$$
	
	$$
	\begin{array}{l l l}
		&wlp(\cmdAssignHloc{\expVar}{\cmdReadHloc{\nextExpVar}},\ 
				\lambda\resVar.\ \postVar
			)
		\\
		=
		&wlp(\cmdLet
						{\varVar}
						{\cmdReadHloc{\nextExpVar}}
						{\cmdAssignHloc{\expVar}{\varVar}}
			)
			&\text{\varVar not free in \expVar}
		\\
		=
		&wlp(\cmdReadHloc{\nextExpVar},\ 
					\lambda\varVar.\
						wlp(\cmdAssignHloc{\expVar}{\varVar},\
									\lambda\resVar.\ \postVar
							)
			)
		\\
		=
		&wlp(\cmdReadHloc{\nextExpVar},\ 
					\lambda\varVar.\
					(
						\slPointsToAny{\expVar} 
							\ \slStar\
							(\slPointsTo{\expVar}{\varVar} \slWand \postVar)
					)
			)
			&\text{$y$ not free in \nextExpVar, \varVar, \expVar, \postVar}
		\\
		=
		&\exists y.\
				\slPointsTo{\nextExpVar}{y}
				\ \wedge\ 
				(
					\slPointsToAny{\expVar} 
					\ \slStar\
					(\slPointsTo{\expVar}{y} \slWand \postVar)
				)
	\end{array}
	$$
	$$
	\begin{array}{l l l}
		&wlp(\cmdAssignHloc
					{\expVar}
					{\cmdReadHloc{\expVar}},\
				\lambda\resVar.\ \postVar
			)
		\\
		=
		&\exists y.\
				\slPointsTo{\expVar}{y}
				\ \wedge\ 
				(
					\slPointsToAny{\expVar} 
					\ \slStar\
					(\slPointsTo{\expVar}{y} \slWand \postVar)
				)
		\\
		\equiv
		&\exists y.\
				\slPointsTo{\expVar}{y}
				\ \wedge\ 
				(
					(
						\slPointsTo{\expVar}{y}
						\ \wedge\
						\slPointsToAny{\expVar} 
					)
					\ \slStar\
					(\slPointsTo{\expVar}{y} \slWand \postVar)
				)
		\\
		\equiv
		&\exists y.\
				\slPointsTo{\expVar}{y}
				\ \wedge\ 
				(
					\slPointsTo{\expVar}{y}
					\ \slStar\
					(\slPointsTo{\expVar}{y} \slWand \postVar)
				)
		\\
		\equiv
		&\exists y.\
		\slPointsTo{\expVar}{y}\ \wedge\ \postVar
	\end{array}
	$$
\end{proof}

\end{document}
