# Supplementary material for: Semi-Automated Modular Formal Verification of Critical Software: Liveness and Completeness Thresholds
Source: arXiv:2403.00934 source file (2024-03-14)
Supplement: Supplementary file 18 [file soap-sec-memory_safety.tex]

\documentclass[../ct4ms-TR-CAV.tex]{subfiles}

\begin{document}

\TodoTextNote{
	Do we still need this notation?
}
\begin{notation}[OLD]
	We denote preconditions by \preVar.
	Further, we aggregate preconditions \preVar and programs \cmdVar into tuples \preProgTuple{\preVar}{\cmdVar}.
\end{notation}

\end{document}
