# Supplementary material for: Semi-Automated Modular Formal Verification of Critical Software: Liveness and Completeness Thresholds
Source: arXiv:2403.00934 source file (2024-03-14)
Supplement: Supplementary file 32 [file appendix.tex]

% !TeX root = ../../thesis.tex
\chapter{This is appendix}\label{ch:appendix}

\ldots

\section{test sec 1}
\chapter{GH stuff}

\section{test sec 2}

%%%%%%%%%%%%%%%%%%%%%%%%%%%%%%%%%%%%%%%%%%%%%%%%%%
% Keep the following \cleardoublepage at the end of this file, 
% otherwise \includeonly includes empty pages.
\cleardoublepage

% vim: tw=70 nocindent expandtab foldmethod=marker foldmarker={{{}{,}{}}}
