# Supplementary material for: Semi-Automated Modular Formal Verification of Critical Software: Liveness and Completeness Thresholds
Source: arXiv:2403.00934 source file (2024-03-14)
Supplement: Supplementary file 33 [file template.tex]

\documentclass[../ct4ms-TR-CAV.tex]{subfiles}


\begin{document}

\end{document}
