# Supplementary material for: Semi-Automated Modular Formal Verification of Critical Software: Liveness and Completeness Thresholds
Source: arXiv:2403.00934 source file (2024-03-14)
Supplement: Supplementary file 34 [file template.tex]

\documentclass[../ghost_signals--paper.tex]{subfiles}

\begin{document}
Hello

\end{document}
